# Supplementary material for: Multi-task longitudinal forecasting with missing values on Alzheimer's Disease
Source: arXiv:2201.05040 source file (2022-01-13)
Supplement: Supplementary file 1 [file appendix.tex]

\newpage
\section{Performance in single task prediction}
\label{sec:AppendixA}

In this section we include the performance of the model in the prediction of V and D, equivalently to Table IV in the manuscript. We compare different imputation strategies in a single variable prediction problem with different sets of input variables depending on the prediction task. 

Table \ref{tab:Ventricle} shows the results obtained when the predicted variable is V. We calculate the MAE on the prediction of Ventricle volume at month 36 using different data information for the months previous to 36. Specifically, V implies that we only use Ventricle volume information on previous time-stamps to predict the value at month 36, Multimodal Data (MD) that we use the rest of the variables and MD + Ventricle that we combine them.
The results show an even more relevant outperformance of the proposed framework, which is capable of predicting the ventricular volume with a MAE of 2,750.

\begin{table}[thp]

\caption{Results obtained in the prediction of Ventricle volume at month 36 using information from baseline to month 24. We used Mean Absolute Error (MAE) score as a performance measure. Columns V, MD and MD+V show the results obtained using only Ventricle volume, MD and both as input, respectively.}
\label{tab:Ventricle}
\centering
\begin{adjustbox}{max width=\columnwidth}
\begin{tabular}{cccccccc}
\toprule
\multirow{2}{*}{Regressor} & Imputation & \multirow{2}{*}{V} & \multirow{2}{*}{MD} & \multirow{2}{*}{MD+V}  \\
& strategy  & &                            &                         &                            \\
\midrule
\multirow{5}{*}{RR}
&\textit{zero}          & 10,291 & 14,241 & 10,312 \\
&\textit{mean}          & 10,291 & 14,241 & 10,312 \\
&\textit{median}        & 10,706 & 14,050 & 10,440 \\
&\textit{most frequent} & 20,902 & 19,832 & 15,753 \\
&\textit{temporal}      & 4,700  & 12,262 & 4,794  \\ \midrule
\multicolumn{2}{c}{SSHIBA}                             & \textbf{2,750} & 16,857 & 2,826 \\
% \multicolumn{2}{c}{SSHIBA}                            & 1988 & 0.977  & \textbf{2750} & \textbf{0.970} & 2826 & 0.969 \\
\bottomrule
\end{tabular}
\end{adjustbox}
\end{table}

Similarly, Table \ref{tab:Diagnosis} shows the results obtained predicting D. This classification problem uses the multilabel AUC as the score and shows an equivalent performance of the analysed algorithms, where the proposed framework greatly outperforms them baselines without temporal imputation. However, the model using only D as input obtains an slight improvement with respect to SSHIBA.

\begin{table}[thp]

\caption{Results obtained in the prediction of Diagnosis at month 36 using information from baseline to month 24. We used multiclass Area Under the Curve (AUC) as a performance measure. Columns D, MD and MD+D show the results obtained using only Diagnosis, MD and both as input, respectively.}
\label{tab:Diagnosis}
\centering
\begin{adjustbox}{max width=\columnwidth}
\begin{tabular}{cccccccc}
\toprule
\multirow{2}{*}{Classifier} & Imputation & \multirow{2}{*}{D} & \multirow{2}{*}{MD} & \multirow{2}{*}{MD+D}  \\
& strategy                             &                         &                           & \\
\midrule
\multirow{4}{*}{LR}
& \textit{zero}          & 0.501 & 0.569 & 0.590 \\
& \textit{mean}          & 0.506 & 0.611 & 0.738 \\
& \textit{median}        & 0.506 & 0.611 & 0.738\\
& \textit{most frequent} & 0.506 & 0.611 & 0.738\\
& \textit{temporal}      & \textbf{0.922} & 0.790 & 0.904\\
% & \textit{KNN}           & 0.534 & 0.724 & 0.738\\
% & \textit{Iterative}     & 0.534 & 0.724 & 0.738\\
\midrule
\multicolumn{2}{c}{SSHIBA}                              & 0.820 & 0.718 & 0.902 \\
\bottomrule
\end{tabular}
\end{adjustbox}
\end{table}
